# Supplementary material for: A fully plasma based electron injector for a linear collider or XFEL
Source: arXiv:2406.04585 ancillary file (2024-06-07)
Supplement: Supplementary file 1 [file supplemental_material.pdf]

# Supplemental Material for "A fully plasma based electron injector for a linear collider or XFEL"

## TRANSVERSE BEAM ELECTRON DYNAMICS IN A PLASMA WAKEFIELD

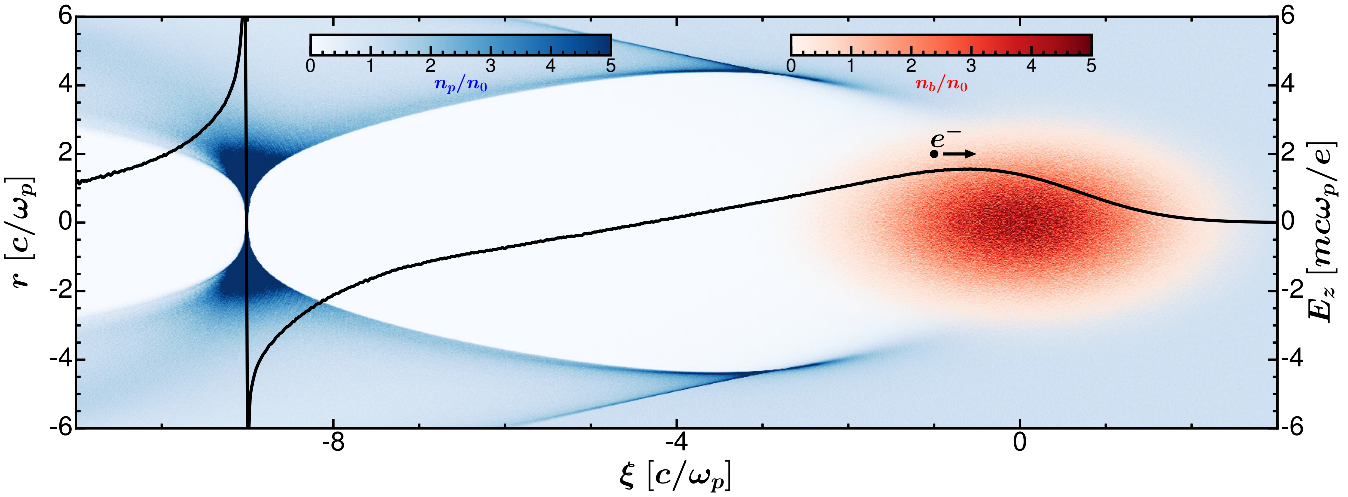


FIG. 1. Plasma wake excited by an electron driver $\{\gamma_b = 20000, \Lambda = 6, k_p\sigma_z = 1, k_p\sigma_0 = 0.5\sqrt{\Lambda}, k_\beta\beta^* = 16\}$ after propagating a distance $z = 60\ c/\omega_p$ in a constant density plasma. The axial electric field $E_z(\xi)$ is plotted in black and sample beam electron with initial phase $(r_i, \xi_i) = (2, -1)$ is annotated with a black dot.

We review the equations governing the motion of a relativistic beam electron ($\vec{v} \simeq c\hat{z}$) propagating in a nonlinear plasma wakefield with uniform density as shown in Fig. 1. For this analysis, we employ normalized units where charge is normalized to $e$, mass to electron mass $m$, velocity to $c$, length to $c/\omega_p$, time to $1/\omega_p$, fields to $mc\omega_p/e$, and potentials to $mc^2/e$. We assume an ultrarelativistic driver ($\gamma_b \gg 1$) is used to excite an azimuthally symmetric wakefield. We also assume the beam electron is fully contained within the ion channel where the focusing force is linear $F_r \approx -r/2$ and the electric field $E_z(\xi)$ does not depend on $r$, where $\xi \equiv z - t$ is the comoving coordinate. Thus, the transverse equation of motion is given by [1, 2]

$$\boldsymbol{x}''(z) + \frac{\gamma_b'(z)}{\gamma_b}\boldsymbol{x}'(z) + k_\beta^2(z)\boldsymbol{x}(z) = 0, \tag{1}$$

where $\boldsymbol{x}(z) = (x(z), y(z))$ represents the transverse coordinates, $\gamma_b$ is the beam particle energy, $k_\beta(z) = 1/\sqrt{2\gamma_b(z)}$ is the instantaneous betatron wavenumber, and primes denote derivatives with respect to $z$. When the particle energy does not change, $\gamma_b' = 0$, the motion is a simple harmonic oscillator $\boldsymbol{x}(z) = \boldsymbol{x_i}\cos(\phi) + \boldsymbol{x_i'}/k_{\beta i}\sin(\phi)$, where $\phi'(z) = k_\beta$ is the betatron phase, and subscript "i" denotes initial values.

When the particle energy $\gamma_b$ changes such that $k_\beta$ varies adiabatically, i.e., $k_\beta' \ll k_\beta^2$, the conservation of $\oint dxp_x$ implies the motion is described by

$$\boldsymbol{x}(z) = \boldsymbol{A_i}\left[\frac{\gamma_{bi}}{\gamma_b(z)}\right]^{1/4}\cos(\phi + \boldsymbol{\phi_i}) \tag{2}$$

$$\boldsymbol{x}'(z) \approx -k_\beta\boldsymbol{A_i}\left[\frac{\gamma_{bi}}{\gamma_b(z)}\right]^{1/4}\sin(\phi + \boldsymbol{\phi_i}). \tag{3}$$

where $\phi(z) = \int_0^z k_\beta(s)ds$, $\boldsymbol{A_i} \approx \sqrt{\boldsymbol{x_i}^2 + \boldsymbol{x_i}'^2/k_{\beta i}^2}$, $\cos\boldsymbol{\phi_i} = \boldsymbol{x_i}/\boldsymbol{A_i}$, and $\sin\boldsymbol{\phi_i} = -\boldsymbol{x_i'}/(k_{\beta i}\boldsymbol{A_i})$. If the density is also changing, this analysis can be generalized [3, 4], but for adiabatic changes in density $\oint dxp_x$ is still conserved.

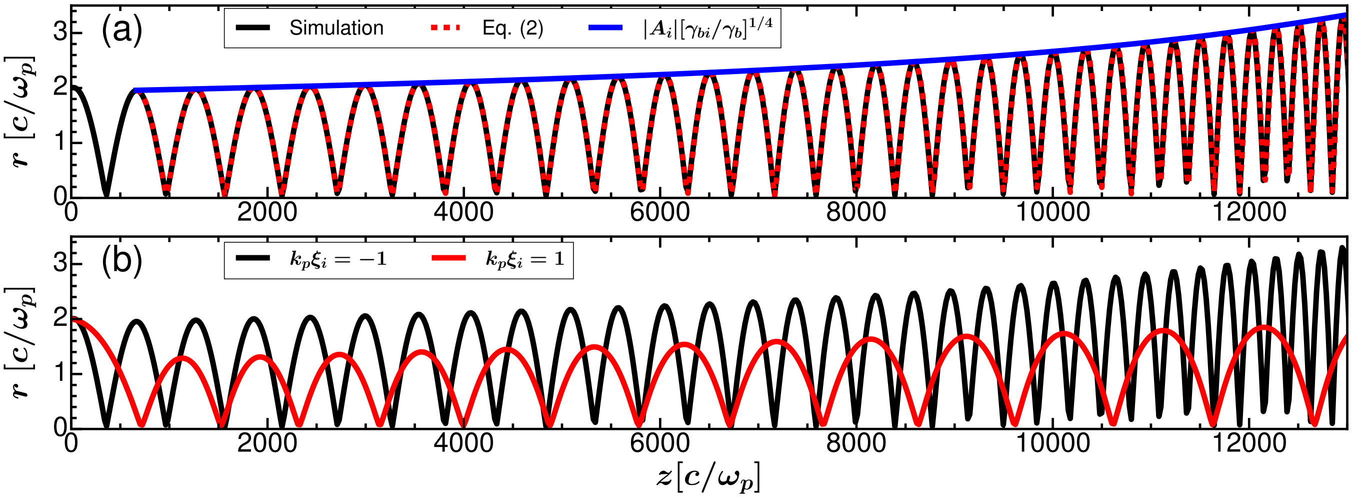


FIG. 2. (a) $r(z)$ (black) of a drive beam particle initially located at $k_p\xi_i = -1$ from the simulation shown in Fig. 1. Eq. (2) and the oscillation amplitude $|\boldsymbol{A_i}|[\gamma_{bi}/\gamma_b]^{1/4}$ are plotted using the simulation data to determine $k_\beta(z)$. Initial conditions of Eq. 2 are evaluated at $k_pz = 660$ after the driver has self-focused. (b) Simulated trajectories of beam particles initially located at $k_p\xi_i = -1$ (black) and $k_p\xi_i = 1$ (red).

Eq. (2) is evaluated for drive beam electrons from Fig. 1 using simulation data to determine the instantaneous betatron wavenumber $k_\beta(z) = 1/\sqrt{2\gamma_b}$. The initial conditions are taken at $k_pz = 660$ at which point the driver has self-focused and the particle's betatron motion is fully contained within the ion channel. The analytical result (dashed red) plotted in Fig. 2(a) exhibits strong agreement with the simulation trajectory (solid black) in terms of periodicity and amplitude. Over long distances, the amplitude (wavelength) adiabatically increases (decreases) as the particle loses energy to the wake and scales with $\gamma_b^{-1/4}$ ($\gamma_b^{1/2}$).

It is worth noting that while Eq. (2) can be applied to most of the beam particles, its underlying assumptions break down at the front of the channel where the plasma is not fully blown out and the focusing force is nonlinear. In these regions, the effective plasma wavenumber varies from 0 to $k_p$ both transversely and longitudinally and beam particles oscillate with betatron frequencies that vary along the driver as shown in Fig. 2(b). The projected spot size is therefore reduced (self-focused) due to emerging spread in the betatron phase. Betatron oscillations at the front ($k_p\xi_i = 1$) are also initially damped as more electrons are blown out and the focusing force increases due to self-focusing. Nevertheless, these particles still exhibit the same characteristics as those in the channel: their oscillation amplitudes gradually increase as they lose energy to the wake.

## LONGITUDINAL BEAM ELECTRON DYNAMICS IN A PLASMA WAKEFIELD

While the beam particles propagate with axial velocity near the speed of light, they can still undergo dephasing over sufficiently long distances. For ultrarelativistic beams ($p_\perp/p_z \ll 1$), the dephasing rate is approximated by Taylor expanding the evolution of the comoving coordinate

$$\frac{d\xi}{dt} = v_z - 1 = \frac{p_z}{\sqrt{1 + p_z^2 + p_\perp^2}} - 1 \approx -\frac{1}{2p_z^2} - \frac{|\boldsymbol{x}'|^2}{2}. \tag{4}$$

where $|\boldsymbol{x}'|^2 = x'^2 + y'^2$. The first term arises from the longitudinal momentum of the beam electron and the second term arises from its transverse divergence described by Eq. (3). Eq. (4) is numerically integrated and plotted (dashed red) in Fig. 3 for the beam particle shown in Fig. 2(a). Strong agreement is observed between the theory and simulation results (black). As the drive beam electron loses energy to the wakefield $E_z(\xi)$ over long distances, the dephasing rate accelerates due to contraction of the betatron wavelength and adiabatic expansion of the transverse oscillation amplitude.

For high energy beam electrons ($\gamma_b \gg 1$), the first term can generally be neglected over a betatron oscillation since it scales as $\gamma_b^{-2}$ while the second term scales as $\gamma_b^{-3/2}$. Thus, the dephasing rate over a single betatron cycle can be

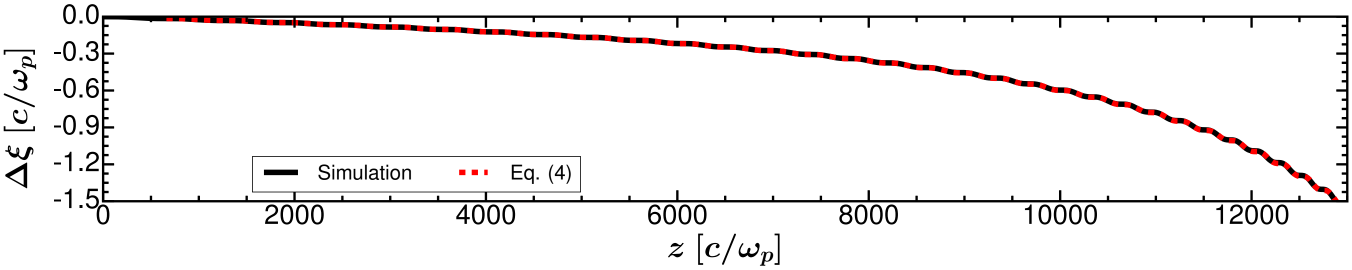


FIG. 3. $\Delta\xi(z) \equiv \xi(z) - \xi(0)$ of the drive beam particle shown in Fig. 2(a) obtained directly from simulation results (black). Eq. (4) is numerically integrated and plotted (dashed red).

approximated by

$$\left\langle \frac{d\xi}{dt} \right\rangle \approx -\frac{\langle |\boldsymbol{x}'|^2 \rangle}{2} \approx -\frac{|\boldsymbol{A_i}|^2}{8}\sqrt{\frac{\gamma_{bi}}{\gamma_b^3}}, \tag{5}$$

where $|\boldsymbol{A_i}|^2 = x_i^2 + y_i^2 + (x_i'^2 + y_i'^2)/k_{\beta i}^2$. The total dephasing rate over some propagation distance can be expressed as

$$\Delta\xi(z) = \int_0^z \left\langle \frac{d\xi}{dt} \right\rangle ds \approx -\frac{|\boldsymbol{A_i}|^2}{8} \int_0^z \sqrt{\frac{\gamma_{bi}}{\gamma_b(s)^3}} ds. \tag{6}$$

Assuming the beam electron experiences some average accelerating (or decelerating) field $\bar{E}_z$ such that we can approximate $d\gamma_b \approx -\bar{E}_z ds$, we find

$$\Delta\xi(z) = -\frac{\boldsymbol{A_i}^2}{8\bar{E}_z} \int_{\gamma_b}^{\gamma_{bi}} \sqrt{\frac{\gamma_{bi}}{\gamma_b^3}} d\gamma_b = -\frac{|\boldsymbol{A_i}|^2}{4\bar{E}_z}\left[\sqrt{\frac{\gamma_{bi}}{\gamma_b}} - 1\right] \tag{7}$$

Substituting $\bar{E}_z = (\gamma_{bi} - \gamma_b)/z$ into Eq. (7), we finally obtain

$$\Delta\xi(z) = \frac{-\boldsymbol{A_i}^2 z}{4\left(\gamma_b + \sqrt{\gamma_b \gamma_{bi}}\right)}. \tag{8}$$

Eq. (8) is compared with $\Delta\xi$ obtained directly from the simulation results after a propagation distance of $z = 13000\ c/\omega_p$ in Fig. 4. Good agreement is observed between the theory and simulations results for particles across

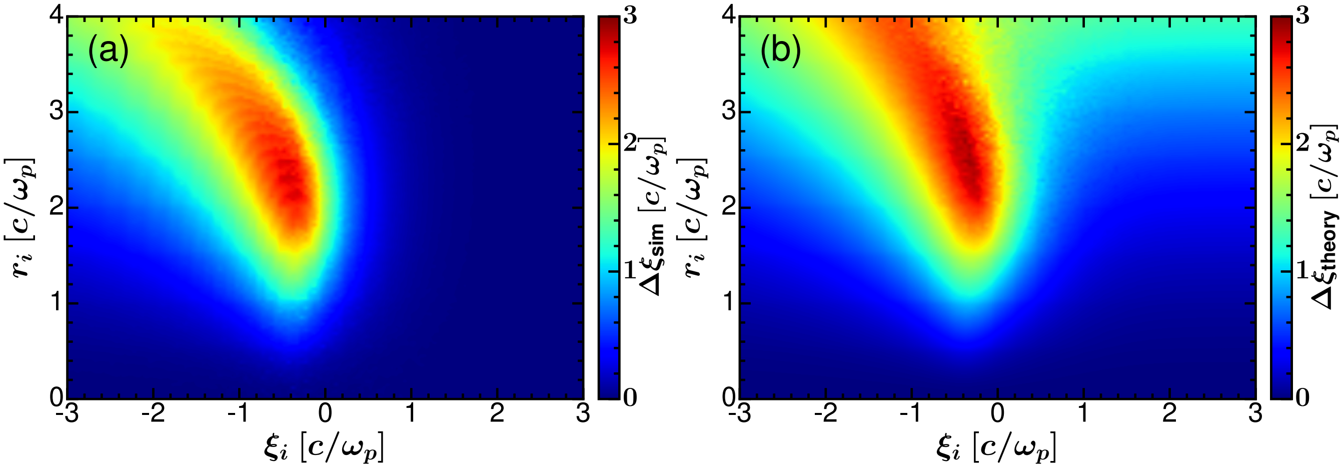


FIG. 4. Contour maps of particle dephasing $\Delta\xi$ obtained from (a) simulation and (b) theory [Eq. (8)] as a function of the initial particle phase space $(\xi_i, r_i)$. The results are generated after a propagation distance of $z = 13000\ c/\omega_p$.

most of the initial phase space $(\xi_i, r_i)$. While Eq. (8) was derived assuming a linear focusing force $F_r/r \approx -1/2$, it still provides reasonable qualitative agreement in regions where plasma electrons are not fully blown out along most of the driver, except at the very front ($\xi_i \gtrsim 1$) where $F_r$ approaches zero.

## DETAILS ON THE MULTI-SHEATH MODEL EQUATIONS

We use multi-sheath model for the wake potential $\psi_0(\xi) = (1+\beta')r_b^2/4$ [5] to calculate the bubble shape $r_b(\xi)$ and electric field $E_z(\xi) = d[\psi_0(r_b)]/d\xi$ from nonlinear theory [1, 2, 5]. Under this model, the plasma source term is described by two plasma sheaths surrounding a fully-cavitated ion channel with radius $r_b(\xi)$. The amplitudes $\{n_1, n_2\}$ and widths $\{\Delta_1, \Delta_2\}$ of the sheaths are modeled as functions of $r_b$ using the same profiles described in Ref. 5,

$$n_2 = n_{20}\exp(-s(r_b/r_m)^t), \quad \Delta_1 = \Delta_{10} + \epsilon r_b, \quad \Delta_2 = \Delta_{20} \tag{9}$$

where $\{n_{20}, s, t, \Delta_{10}, \epsilon, \Delta_{20}\}$ are constants and $r_m$ is the maximum bubble radius. $n_1 = \frac{r_b^2 - n_2(\Delta_2^2 + 2\Delta_2\Delta_1 + 2\Delta_2)}{(r_b+\Delta_1)^2 - r_b^2}$ is constrained by the conservation of charge, and $n_{20} = \frac{2\psi_{min}}{(\Delta_{10}+\Delta_{20})^2 \ln\left(1+\frac{\Delta_{20}}{\Delta_{10}}\right)}$ is constrained by the minimum wake potential. The sheath function is therefore given by $\beta' = 2(1+n_1)\ln[1+\frac{\Delta_1}{r_b}] - 1 + 2n_2(1+\frac{\Delta_1+\Delta_2}{r_b})^2\ln[1+\frac{\Delta_2}{r_b+\Delta_1}]$. It is worth noting $\beta'(r_b, n_1, n_2, \Delta_1, \Delta_2)$ permits negative values for the wake potential through the parameter $\psi_{min}$. The differential equation for $r_b(\xi)$ is described by [5]

$$A'(r_b)\frac{d^2 r_b}{d\xi^2} + B'(r_b) r_b \left(\frac{dr_b}{d\xi}\right)^2 + C'(r_b) r_b = \frac{\lambda(\xi)}{r_b}, \tag{10}$$

where $A'(r_b) = 1 + [\frac{1}{4} + \frac{\beta'}{2} + \frac{1}{8}r_b\frac{d\beta'}{dr_b}]r_b^2$, $B'(r_b) = \frac{1}{2} + \frac{3}{4}\beta' + \frac{3}{4}r_b\frac{d\beta'}{dr_b} + \frac{1}{8}r_b^2\frac{d^2\beta'}{dr_b^2}$, $C'(r_b) = \frac{1}{4}[1 + \frac{1}{(1+\beta' r_b^2/4)^2}]$, $\lambda(\xi) = 4\pi r_e \int_0^{r_b} n_b(\xi, r) r dr$. Eq. (10) is numerically integrated from maximum bubble radius $r_b(\xi_m) = r_m$ to the rear of the channel $r_b = 0$. Once $r_b(\xi)$ is determined, the electric field $E_z(\xi) = -D'(r_b) r_b \frac{dr_b}{d\xi}$ can be calculated, where $D'(r_b) = \frac{1}{2} + \frac{\beta'}{2} + \frac{1}{4}r_b\frac{d\beta'}{dr_b}$.

For the drive beam parameters $\{\gamma_b = 20000, \Lambda = 6, k_p\sigma_z = 1, k_p\sigma_0 = 0.5\sqrt{\Lambda}, k_\beta\beta^* = 16\}$, we use the integration parameters $\{s = 3, t = 3, \Delta_{10} = 1, \epsilon = 0.05, \Delta_{20} = 3\}$ for all propagation distances. The minimum wake potential $\psi_{min} \approx -1$ ($-0.93$) used at $k_p z = 4000$ (12500) is obtained directly from the PIC simulation results.

[1] W. Lu, C. Huang, M. Zhou, M. Tzoufras, F. S. Tsung, W. B. Mori, and T. Katsouleas, Physics of Plasmas **13**, 056709 (2006).
[2] W. Lu, C. Huang, M. Zhou, W. B. Mori, and T. Katsouleas, Phys. Rev. Lett. **96**, 165002 (2006).
[3] Y. Zhao, W. An, X. Xu, F. Li, L. Hildebrand, M. J. Hogan, V. Yakimenko, C. Joshi, and W. B. Mori, Phys. Rev. Accel. Beams **23**, 011302 (2020).
[4] R. Ariniello, C. E. Doss, V. Lee, C. Hansel, J. R. Cary, and M. D. Litos, Phys. Rev. Res. **4**, 043120 (2022).
[5] T. N. Dalichaouch, X. L. Xu, A. Tableman, F. Li, F. S. Tsung, and W. B. Mori, Physics of Plasmas **28**, 063103 (2021), https://doi.org/10.1063/5.0051282.
